# Supplementary material for: Real-time polarimetry of hyperpolarized $^{13}$C nuclear spins using an atomic magnetometer
Source: arXiv:2301.06607 source file (2023-09-12)
Supplement: Supplementary file 1 [file 26-SI.pdf]

# Real-time polarimetry of hyperpolarized $^{13}$C nuclear spins using an atomic magnetometer

## Supporting Information

**Kostas Mouloudakis[a], Marc Azagra[b], S Bodenstedt[a], Irene Marco-Rius[b], Morgan W. Mitchell[a,c], Michael C. D. Tayler[a,*]**

[a] *ICFO-Institut de Ciències Fotòniques, The Barcelona Institute of Science and Technology, 08860 Castelldefels (Barcelona), Spain.*

[b] *IBEC – Institute for Bioengineering of Catalonia, 08028 Barcelona, Spain*

[c] *ICREA – Institució Catalana de Recerca i Estudis Avançats, 08010 Barcelona, Spain.*

[*] *Corresponding author. Email: michael.tayler@icfo.eu*

## Contents

S.1 Experimental detail . . . 2
S.1.1 Magnetic shielding . . . 2
S.1.2 Atomic magnetometer . . . 2
S.1.3 Piercing solenoid . . . 3
S.1.4 Pulsed field control . . . 3
S.1.5 Additional notes . . . 3

## S.1 Experimental detail

The magnetic field of the nuclear-spin-polarized liquid sample was detected using the experimental setup illustrated in Figure S1 and Figure S2. Main parts of the setup are described in the following subsections.

### S.1.1 Magnetic shielding

A commercial magnetic shield was used to passively screen background magnetic fields in the laboratory, up to several mT in magnitude, down to a residual of between 10 and 30 nT. The shield comprised three concentric outer layers of MuMetal and one innermost layer of ferrite (MS-1LF, Twinleaf LLC). The shield as receiver from the manufacturer also contained a set of XYZ printed-circuit coils on a flexible polyimide film attached to the interior of the ferrite layer, as shown in the Figure S1(b). These coils are normally intended to be used to supply compensatory magnetic fields along $x$-, $y$- and $z$-axes to achieve zero residual magnetic field inside the shield. In the present work, the $x$- and $y$-axis coils were used to supply the XY4 pulses (indicated in Figure 1 of the main manuscript) and the $z$-axis coil (Z) was unused. Field-to-current ratios were 69 nT/mA for the X coil and 130 nT/mA for the Y coil.

### S.1.2 Atomic magnetometer

A linearly polarized 1 mW laser beam was generated by a vertical-cavity surface-emitting laser at the $^{87}$Rb $D_1$ transition wavelength, around 795 nm. The beam was passed through a Keplerian telescope to adjust its width to around 3 mm and then a zero-order quarter-wave plate to generate circularly polarized light. The light then passed into the magnetic shield through the end hole and then through an optically dense alkali medium enclosed in a MEMS vapor cell. Cell external dimensions were 5 mm by 10 mm by 1.5 mm and internal path length 1 mm. The cell was locally heated to a temperature of around 150 °C using a resistive heater. The beam passing through the vapor was detected outside the magnetic shield, where it was focused on a low-noise amplified photodetector (Thorlabs model PDA36A2) and the resulting output voltage sampled using a 24-bit analog-to-digital converter integrated circuit at 48 ksps (Cirrus Logic CS4272) interfaced with a microcontroller (ARM Cortex M4F).

To operate the above apparatus as a magnetometer, the local magnetic field at the atomic vapor cell was modulated by applying a sinusoidal field along the $z$ direction of 20 nT in amplitude and approximately 500 Hz in frequency. The field was supplied using a miniature biplanar printed-circuit coil set[1] positioned around the cell oven, as shown in Figure S1(b) in green. During modulation, the photodetector signal was sampled using the CS4272 and demodulated at the same frequency, then digital lowpass filtered to produce a quadrature signal whose amplitude was proportional to the dc bias field $B_z$. This field was the sum of the residual field inside the magnetic shield and the nuclear magnetic field of the hyperpolarized sample, seen at the position the atoms.

### S.1.3 Piercing solenoid

A 10-inch-long, 10-mm-o.d., 8.5-mm-i.d. flat-bottomed glass tube was used to contain the NMR sample during the magnetometry measurements. This was wrapped along its length with 0.15 mm diameter enameled copper wire to form a single layer solenoid coil, which when energized supplied a 30 µT bias field along the $z$ axis; this field ensured that the spin polarization was always parallel to $z$, even when the sample was transported in and out of the magnetic shield. The bottom of the tube/solenoid structure sat atop the magnetometer oven as shown in Figure S1(b).

### S.1.4 Pulsed field control

The alternating $(\pi)_x \equiv (\pi/2)_x(\pi)_y(\pi/2)_x$ and $(\pi)_y \equiv (\pi/2)_y(\pi)_{-x}(\pi/2)_y$ composite pulses constituting the XY4 pulse sequence shown in Figure 1 of the main paper were applied via bidirectional switching of direct current in the X and Y coils, as shown schematically in Figure S2. Current switching in both of the coils was performed using a dual-channel H-bridge circuit (Toshiba TB6612FNG on Pololu carrier board). The logic lines of the H-bridge circuit were controlled using the M4F microcontroller's digital input-output and were asynchronous with CS4272 data acquisition. The approximate duration of each $\pi$ composite pulse was 50 µs on $^1$H for a peak current of 0.5 A.

### S.1.5 Additional notes

The table-top setup involving the magnetic shield, magnetometer and control electronics was constructed at ICFO and transported to IBEC in the rear passenger seat of a car belonging to one of the authors. The experiments described in the main manuscript were then performed at IBEC in the same laboratory as a commercial dissolution-DNP polarizer (HyperSense, Oxford Instruments Ltd.), as shown in Figure S1(a), on a vibrationally undamped table located approximately 1 m away from the polarizer magnet. The distance was chosen so that the magnetometer would be as close as possible to the polarizer without impeding access to its working parts.

## References


[1] MCD Tayler, K Mouloudakis, R Zetter, D Hunter, VG Lucivero, S Bodenstedt, L Parkkonen and MW Mitchell, "Miniature biplanar coils for alkali-metal-vapor magnetometry", *Phys. Rev. Applied* **18**, 014036 (2022).

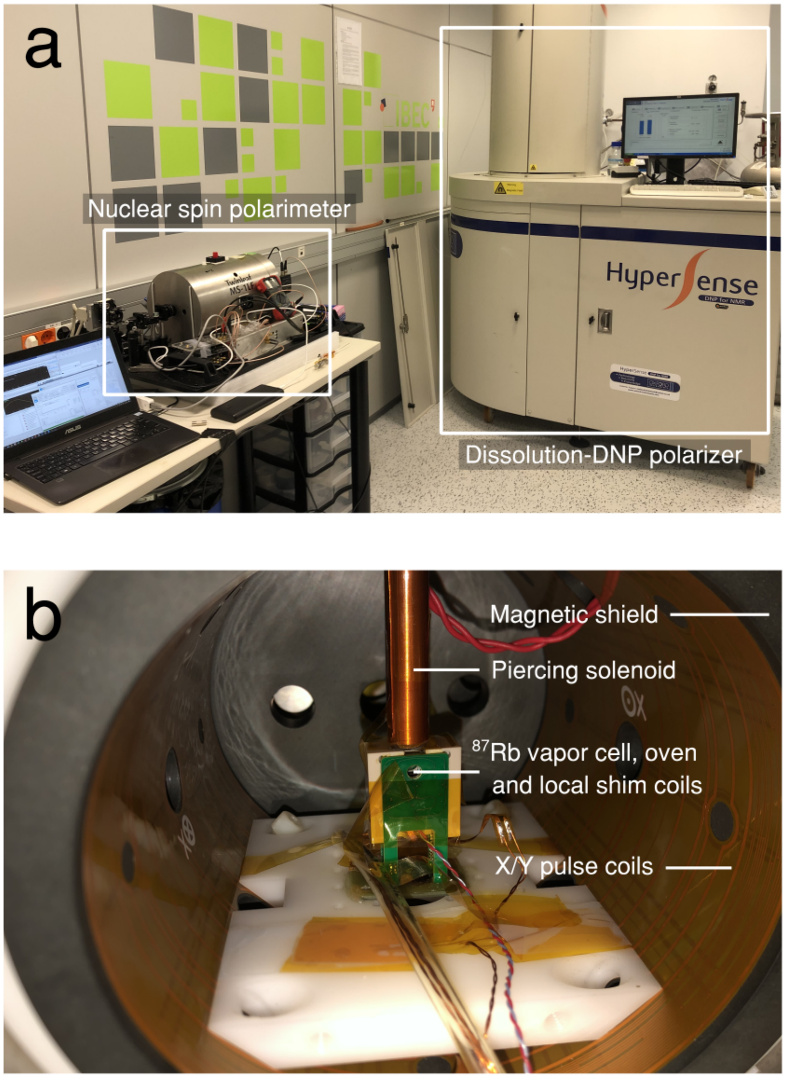


Fig. S1: Photographs of the experimental apparatus in use at the molecular-imaging-for-precision-medicine group at the Catalonia Institute for Bioengineering (IBEC): (a) the nuclear spin polarimeter, on top of a table approximately 1 m away from a commercial dissolution-DNP polarizer. The main visible feature of the setup is the cylindrical MuMetal magnetic shield; (b) a view of the interior of the magnetic shield, containing the coils for XY4 pulses on a flexible printed circuit board, the magnetometer, and a solenoid coil that surrounds the sample tube containing hyperpolarized liquid. A schematic version of (b) appears in the lower part of Figure S2 .

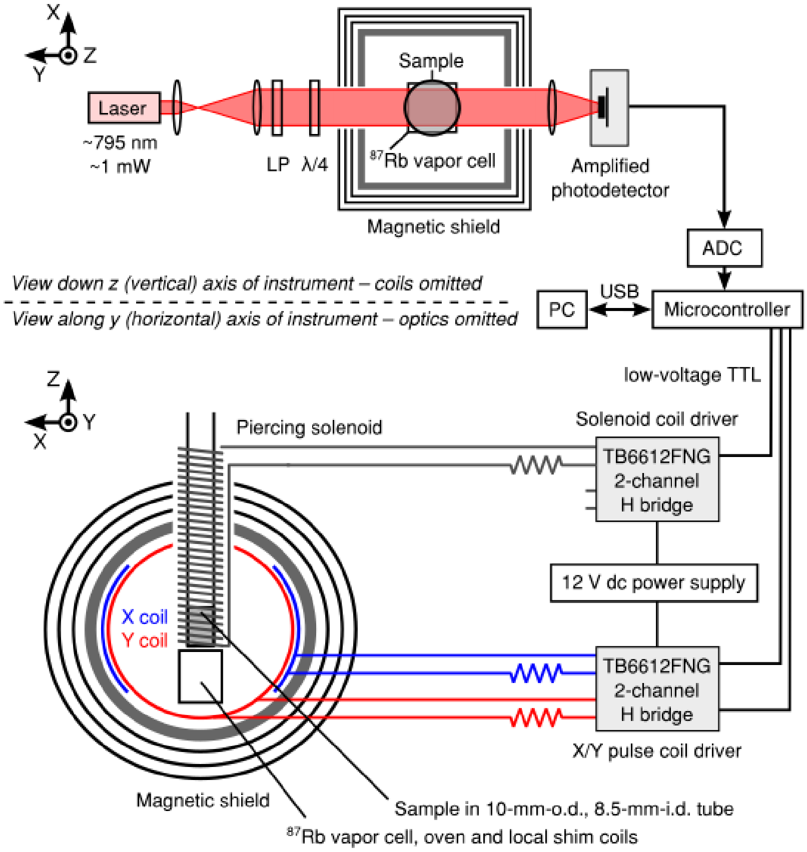


Fig. S2: Schematic view of the experimental setup for real-time nuclear spin polarimetry. The top half of the figure illustrates the magnetically shielded portion of the setup from a vertical point of view, down the $z$ axis. The bottom half shows the view along the $y$ axis, parallel to the laser beam.
